# Supplementary material for: First-Principles Study of Recombination-Enhanced Migration of an Interstitial Magnesium in Gallium Nitride
Source: arXiv:2402.06214 source file (2024-05-02)
Supplement: Supplementary file 1 [file Suppl.pdf]

# Supplementary Material: First-Principles Study of Recombination-Enhanced Migration of an Interstitial Magnesium in Gallium Nitride

Yuansheng Zhao,[1] Kenji Shiraishi,[1,2] Tetsuo Narita,[3] and Atsushi Oshiyama[1]
[1)] *Institute of Materials and Systems for Sustainability, Nagoya University, Nagoya 464-8603, Japan*[a)]
[2)] *Graduate School of Engineering, Nagoya University, Nagoya 464-8601, Japan*
[3)] *Toyota Central R&D Labs., Inc., Nagakute, Aichi 480-1192, Japan*

## I. CALCULATION DETAILS

First-principles DFT calculations have been performed with the Vienna ab initio Simulation Package (VASP)[1,2] with the projector-augmented potentials[3] simulating nuclei and core electrons. Generalized gradient approximation (GGA) of Perdew, Burke and Ernzerhof (PBE)[4] for the geometry optimization and hybrid approximation of Heyd, Scuseria and Ernzerhof (HSE)[5] for the electronic-structure and the total-energy calculations for the optimized geometries, are used to the exchange-correlation energy. Throughout the whole calculation, we do not explicitly treat the 3$d$ electrons of Ga following previous similar studies[6,7].

The primitive cell optimization with the cutoff energy of 400 eV for the plane-wave basis set and an $8 \times 8 \times 8$ $\boldsymbol{k}$-point mesh yields the lattice constant of $a = 3.23$Å and $c = 5.25$Å which agree with the experimental value with an error of $\sim 1\%$. The experimental band gap of crystalline GaN of 3.4 eV can be reproduced in the present hybrid approximation with the mixing parameter $\alpha = 0.34$ and range-separation parameter $\omega = 0.2\text{Å}^{-1}$ of Fock exchange. An Mg interstitial is embedded in a $4 \times 4 \times 3$ supercell and is optimized using $2 \times 2 \times 2$ $\boldsymbol{k}$-point mesh until the force acting on each atom is smaller than $0.01\,\text{eV}\cdot\text{Å}^{-1}$. While sampling the Brillouin zone using $\Gamma$ point only can converge the formation energy at +2 charge states, for $q = +1$ or 0, using $2\times2\times2$ $\boldsymbol{k}$-point mesh is required.

Spin-polarized calculations shows that all the structures with $q = +2$ or 0 are not spin polarized at both PBE and HSE levels. In the case of $q = +1$, at HSE level, all valid states (no electrons on conduction band) has spin 1/2, where spin-up electrons are filled up to the valence band top (VBT) plus the gap state across the Brillouin zone while spin-down electrons are filled up to VBT. However, at PBE level, due to the underestimation of band gap, the energy of gap state and conduction band overlap, resulting in partial occupation in conduction band for spin-down electrons. We believe that the HSE is more accurate and therefore, during structural optimizations, we fix the band occupation numbers to those found in HSE calculations. This can further optimize the structures, improving the final energy calculated using HSE by as much as 0.2 eV.

For determination of migration pathways between the stable and metastable configurations, we use the nudged elastic band (NEB) method with improved tangential estimate[8] implemented by the Transition State Tools for VASP (VTST)[9]. We use 7 images between the initial and final structures and the $\boldsymbol{k}$-point mesh and convergence criterion are the same as above. We confirmed that there are no kinks formed in the converged pathways by checking the angles between each image and the equidistance condition is satisfied with relative deviation $< 10^{-5}$. In Fig. 4 of the main text, the blue, red and green dots are the result of calculation connecting the O site and metastable sites [$(\text{MgGa})_{\text{ic}}$, $\text{Mg}_{\text{Ga}}\text{Ga}_{\text{i}}$ or T] at charge state +2, +1 and 0, respectively. For $q = +1$ or 0, near the O site (small $\xi$), the additional electrons occupy the conduction band and the energies of these invalid structures are not shown. It is noteworthy that by setting the charge state of each image individually, the variation of the charge states during the migration process can be simulated and the results are shown by the empty squares in Fig. 4 of the main text.

## II. ADDITIONAL FIGURES

The top views of the structures shown in Fig. 1 and 3 of the main text are shown in Fig. S1 and S2, respectively.

[1] G. Kresse and J. Furthmüller, Physical Review B **54**, 11169 (1996).
[2] G. Kresse and D. Joubert, Physical Review B **59**, 1758 (1999).
[3] P. E. Blöchl, Physical Review B **50**, 17953 (1994).
[4] J. P. Perdew, K. Burke, and M. Ernzerhof, Physical Review Letters **77**, 3865 (1996).
[5] J. Heyd, G. E. Scuseria, and M. Ernzerhof, The Journal of Chemical Physics **118**, 8207 (2003).
[6] G. Miceli and A. Pasquarello, Physica Status Solidi (RRL)–Rapid Research Letters **11**, 1700081 (2017).
[7] G. Miceli and A. Pasquarello, Physical Review B **93**, 165207 (2016).
[8] G. Henkelman and H. Jónsson, The Journal of Chemical Physics **113**, 9978 (2000).
[9] Transition State Tools for VASP: https://theory.cm.utexas.edu/vtsttools/.

[a)] Electronic mail: zhao.yuansheng.u3@f.mail.nagoya-u.ac.jp

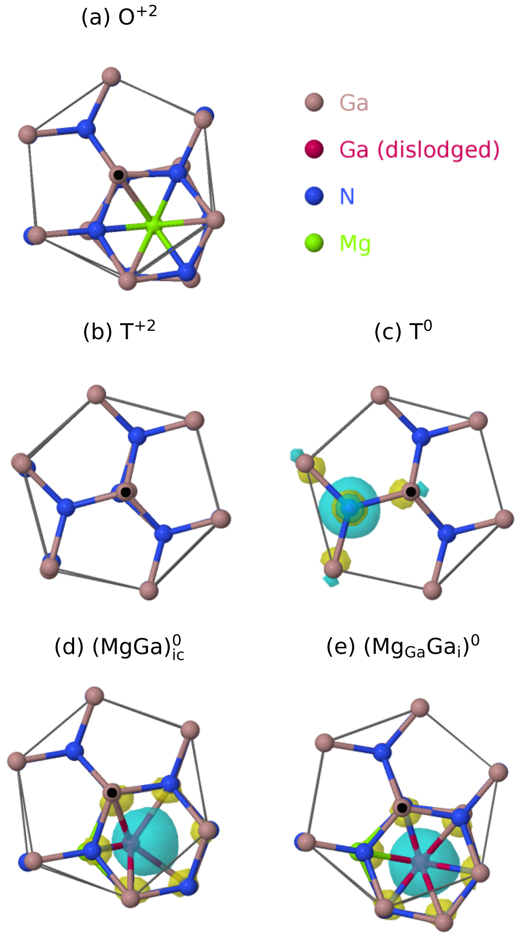


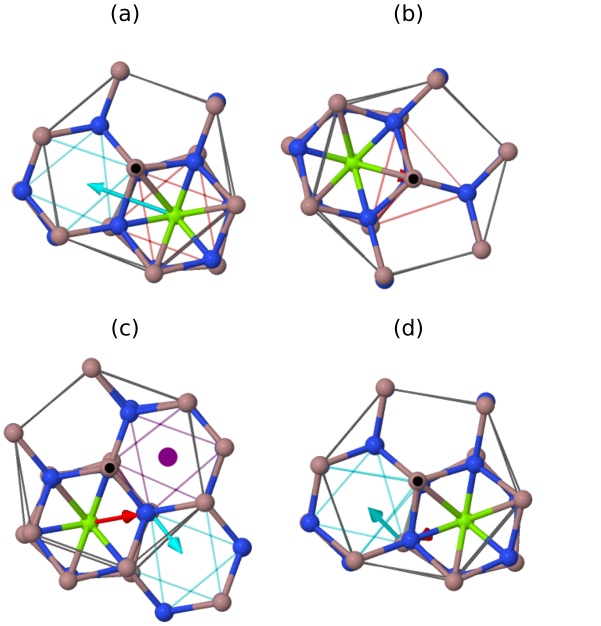


FIG. S1. Stable and metastable configurations of interstitial Mg in GaN (Fig. 1 in the main text), viewed from the $c$ axis: **(a)** $\mathrm{O}^{+2}$, **(b)** $\mathrm{T}^{+2}$, **(c)** $\mathrm{T}^{0}$, **(d)** $(\mathrm{MgGa})^{0}_{\mathrm{ic}}$, and **(d)** $(\mathrm{Mg_{Ga}Ga_{i}})^{0}$ configurations. For the last three, the wavefunction of the gap state is also shown with the value for the isosurface being 40% of the maximum. It is noteworthy that the Mg and the nearest-neighbor Ga are found to be located in the $(1\bar{1}00)$ plane in (d) and (e).

FIG. S2. Migration pathways (Fig. 3 in the main text), viewed from the $c$ axis: **(a)** $\mathrm{OO}^{z}$ and $\mathrm{OO}^{x}$ paths, **(b)** OT path, **(c)** $\mathrm{O(MgGa)}^{1}_{\mathrm{ic}}$ path, and **(d)** $\mathrm{O(MgGa)}^{2}_{\mathrm{ic}}$ path and $\mathrm{O(Mg_{Ga}Ga_{i})}$ path.
